# Supplementary material for: Tracking Large-Scale Video Remix in Real-World Events
Source: arXiv:1210.0623 source file (2013-05-12)
Supplement: Supplementary file 1 [file appendix.tex]

\newpage

\section{Appendix}

\secmoveup
\subsection{Meme frequency distribution}
\label{ssec:wfreq}

In addition to detection performance, we evaluate the quality of
detected memes by studying their frequency distribution and comparing
it with the word frequency distribution. Figure~\ref{fig:memedata4}(d) shows the textual word
and visual meme frequencies shown in a log-log scale.
Performing a regression fit, we obtain the following Zipf's
power law distributions:
$$f(w_t) \propto r^{1.102};~f(w_v) \propto r^{1.959} $$
The exponent $s$ for words in the title and description is close to
that of English words ($\sim1.0$). For visual memes \mbox{$s=1.959$},
suggesting that the diversity of visual memes is less than that of
words at the lower-frequency end.  Still, Figure~\ref{fig:memedata4}(d)
validates that the visual memes form a vocabulary with a ``proper''
distribution and can be used as visual words for topic modeling,
jointly with the textual words.

\begin{figure}[tb]
\centering \includegraphics[angle=0,width=0.48\textwidth]{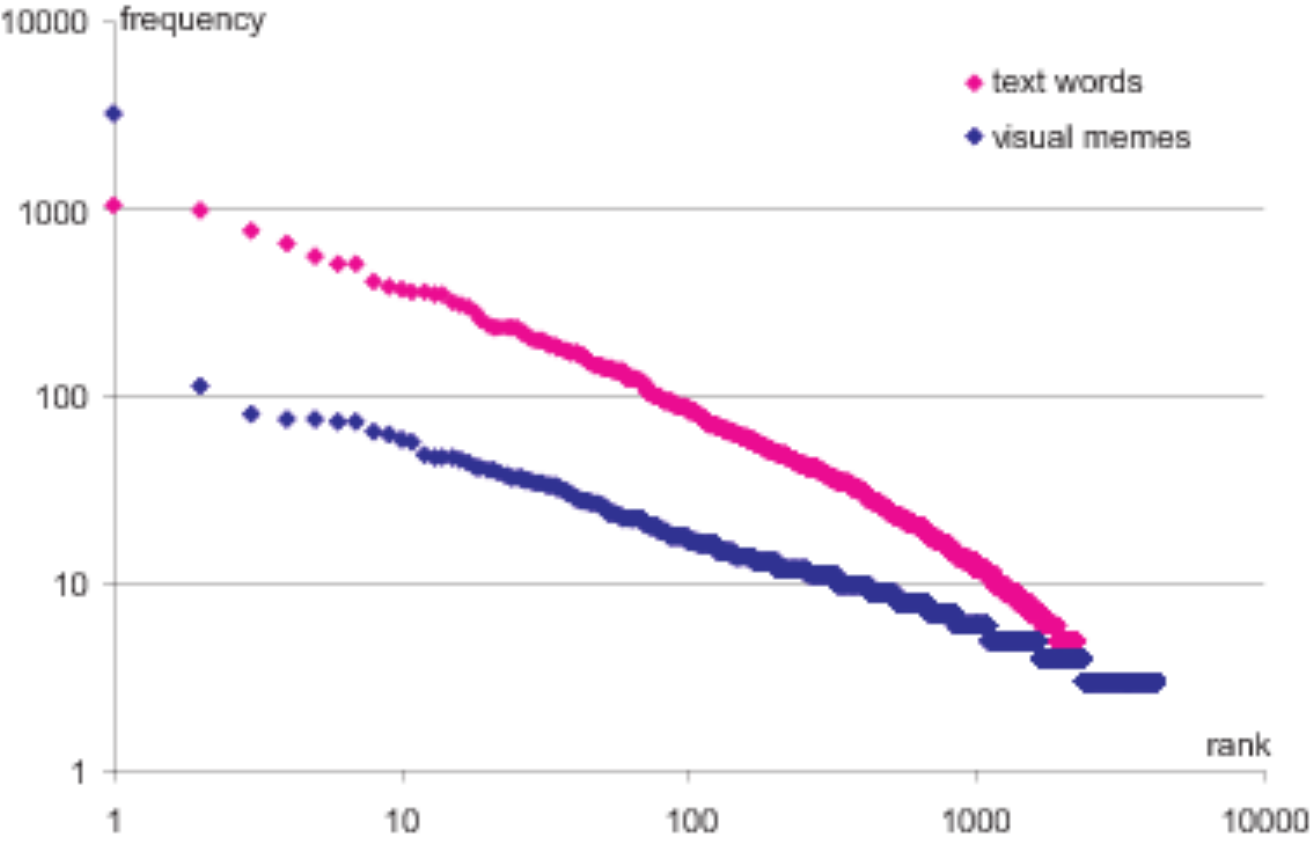}
\caption{Content reposting probability.}
\label{fig:wfreq}
\end{figure}

\secmoveup
\subsubsection{Content originators and aggregators}
\textmoveup

\begin{figure}[tbh]
%\begin{minipage}[t!]{0.55\linewidth}
%  \centering \includegraphics[angle=0,width=\textwidth,height=2.5in]{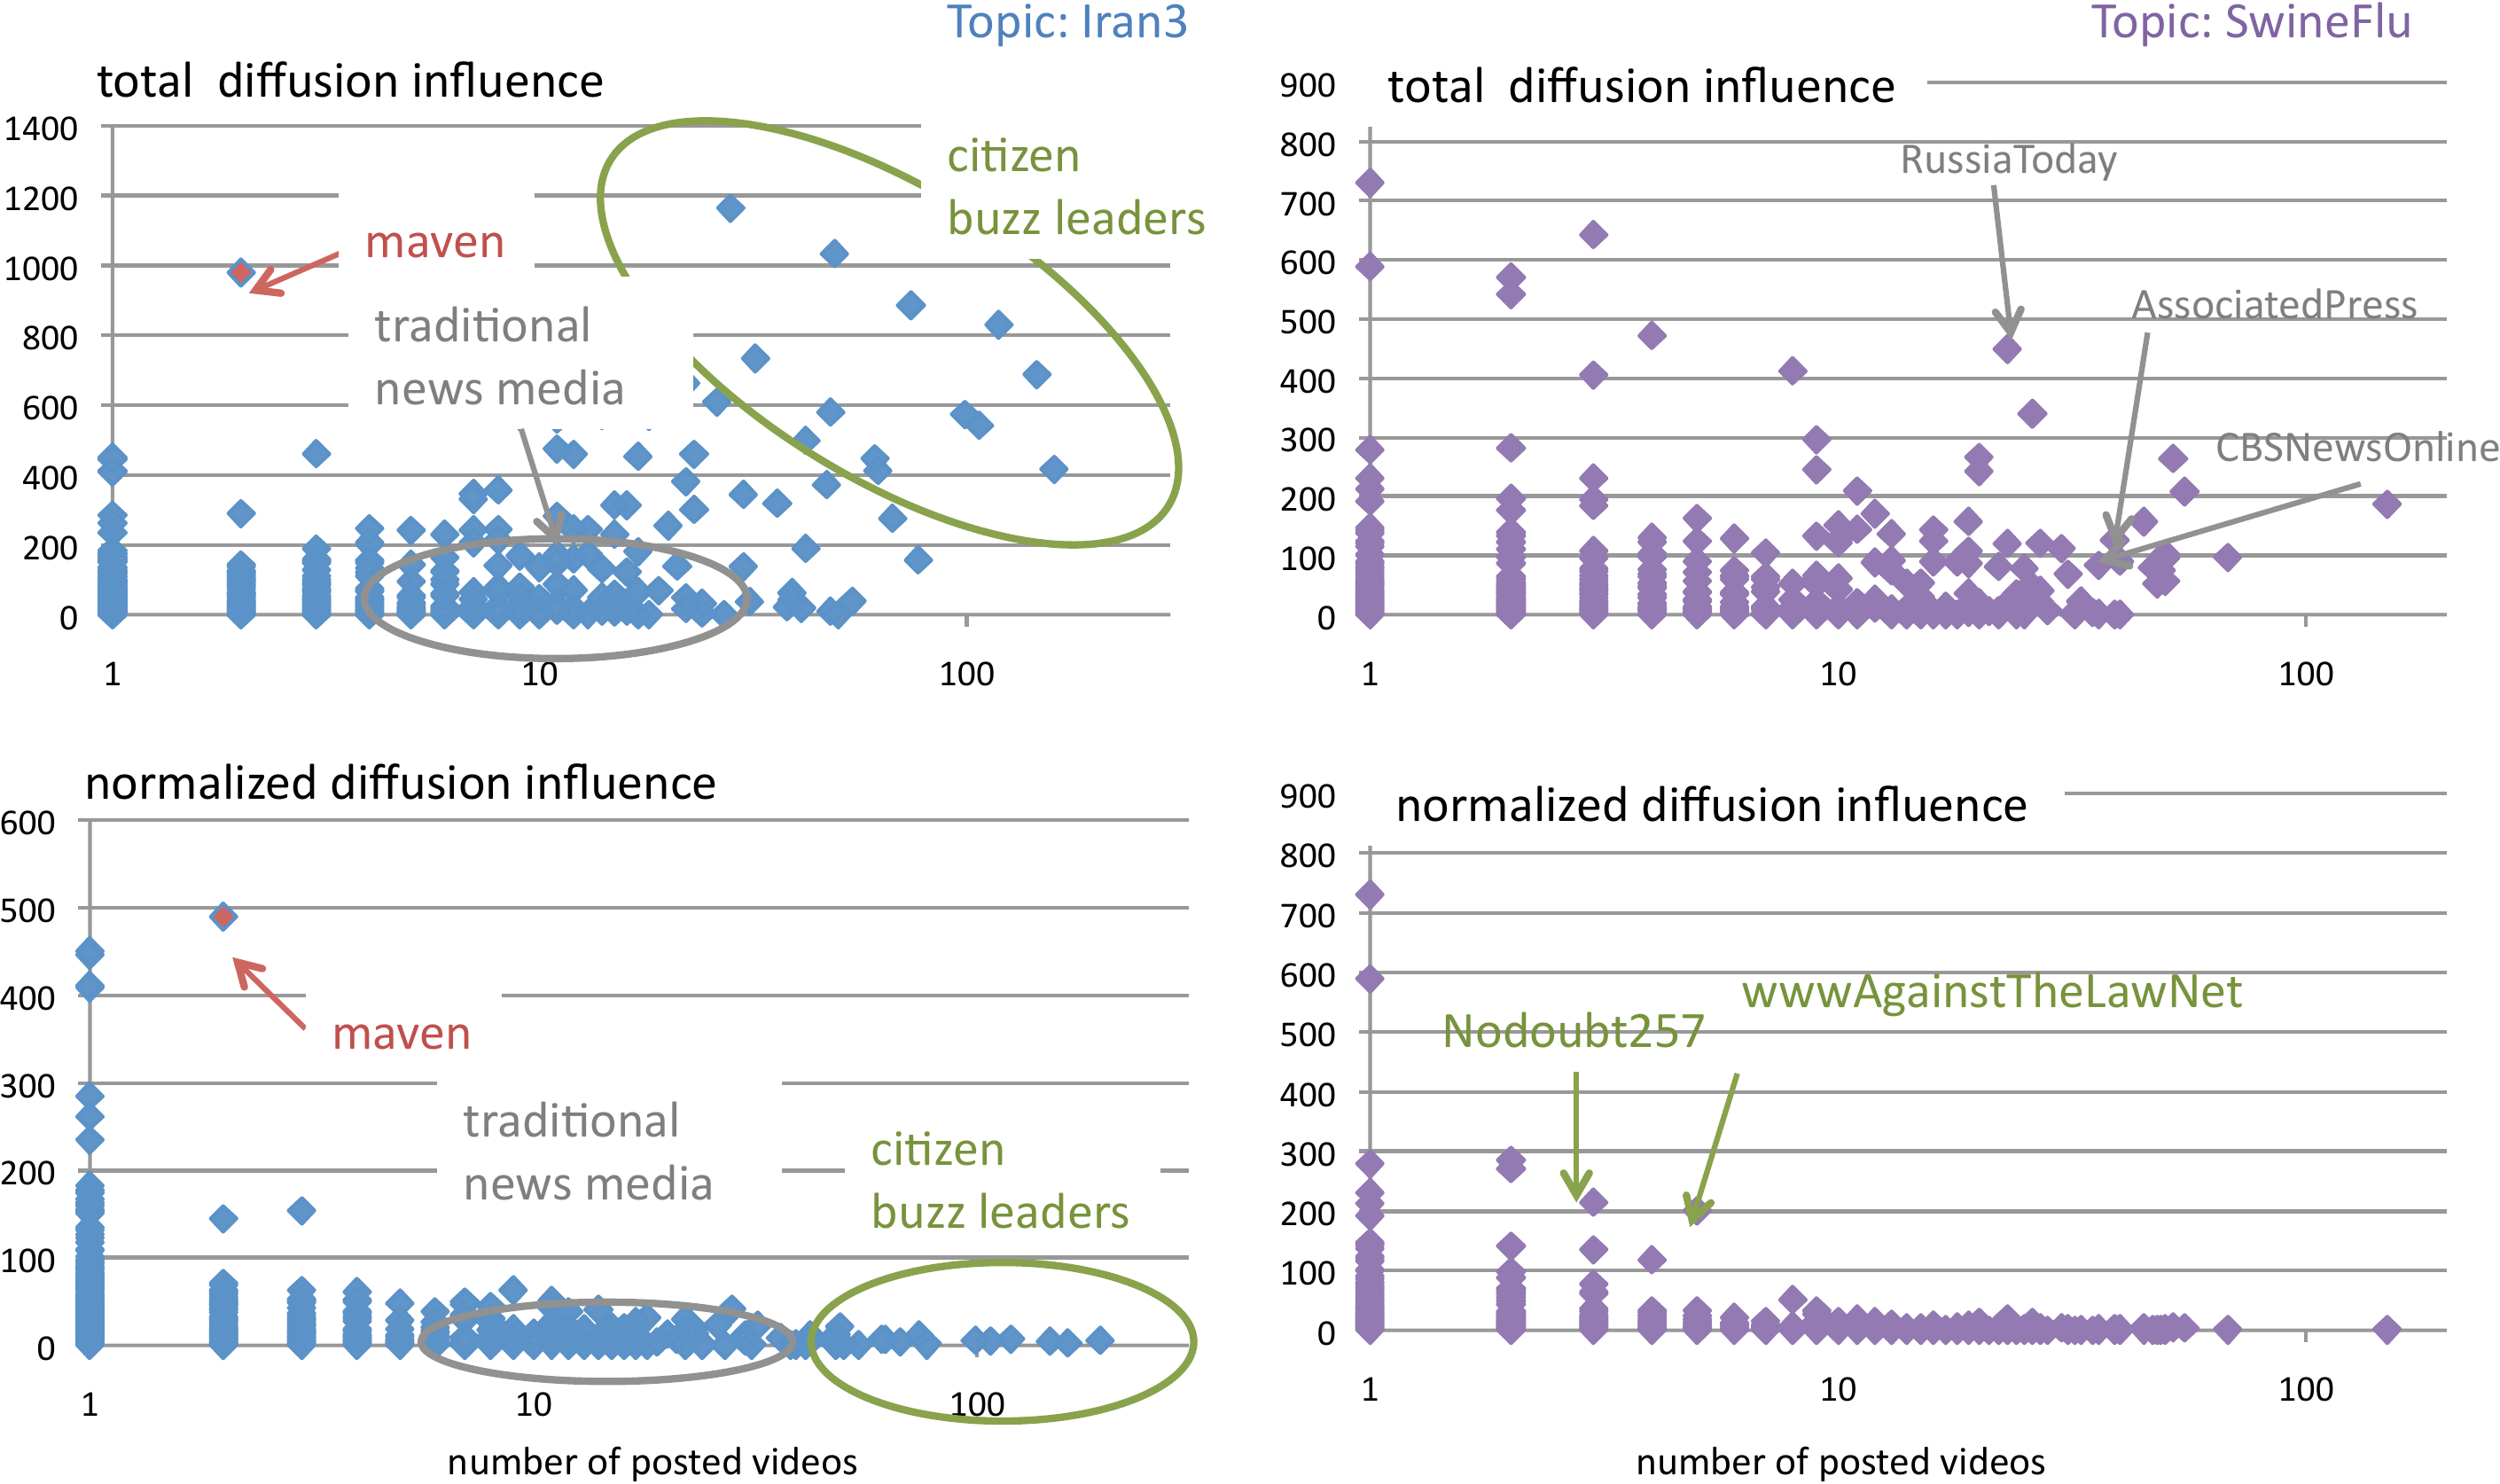}
%  \caption{The diffusion index (Sec~\ref{ssec:diffuidx}). Left: Iran topic (dataset B), Right: Swine Flu
%    (dataset A). }
%  \label{fig:diffusion}
%\end{minipage}
%\hfill
%\begin{minipage}[t!]{.42\linewidth}
  \centering \includegraphics[angle=0,width=.48\textwidth]{fig/originators}  % ,height=2.5in
  \caption{Content originators vs news aggregators.}
  \label{fig:originators}
%\end{minipage}
\end{figure}

Figure~\ref{fig:diffusion} shows that the role of traditional media vs. social media and citizen journalism can vary substantially across
topics. It also suggests that the authors' diffusion score---and therefore overall influence---is only partially correlated to the number
of videos they produce.  In other words, an author can become influential by producing a small number of original videos that induce many
follow-on memes (e.g., the ``maven'' user), or an author can become influential by discovering and re-posting many pieces of other people's
content early in the meme lifecycle. Both types of authors have an important role in the overall evolution and influence of a piece of
content.  We call these hypothetical author types {\em
  content originators} and {\em content aggregators}, and we attempt
to discriminate between them using an {\em author originality index},
defined as the fraction of video memes first originated by a given
author over the total number of video memes the author participates in
(originated or re-posted). 
%This ratio ignores videos that have not been re-posted at all.

In order to compute this index, we consider all meme clusters on the Iran dataset B.  We exclude clusters without a clear
originator (i.e., when multiple videos containing the same meme are posted within the first hour the meme is observed). This excludes some
legitimate memes from the analysis but reduces noise due to incorrect meme cluster fragmentation.  The remaining memes are
used to tally up votes for each author in terms of how many times they were first to post a meme versus they re-posted a known meme.  This
produces a set of 235 ``originators'' and 1258 ``aggregators''.

The author originality index against author productivity is shown on
Figure~\ref{fig:originators}, it clearly identifies content originator
and content aggregator users, and further shows that traditional media
was neither.  In fact, most traditional media sources represented in
this dataset had very low originality index scores, apparently due to
the media blackout imposed by the Iranian regime during the
protests.  Another user that pops up as an interesting outlier is
a mix between an originator and an aggregator, and turns out to be a
controversial radio show host, Alex Jones, who had a series of
YouTube videos discussing potential US involvement in Iran.

\secmoveup
\subsection{Content freshness}
\label{ssec:yt-memory}\textmoveup

We conduct a ``memory experiment'' to evaluate the age of the returned videos from YouTube,
 i.e., content {\em freshness}. This can be used to determine the extend of influence on video
 remixing from past entries. We ran the querying and content extraction during one single day,
 $d_0$=`2010-04-04', across a set of seven diverse
 topics spanning environment, health, economics and international politics.
 Figure~\ref{fig:memory}(top) shows the unique video entries returned for each topic, and
 Figure~\ref{fig:memory}(bottom) shows the fraction of videos as a function of its age (the interval
 between its upload date and $d_0$, averaged over all seven topics. We note that the content
 volume is significant for any of these topics (1800--6500), and that the age distribution
 is approximately power law, as observed in related studies~\cite{crane2008viral}. We obtain a power-law
 regression fit for the content volume versus age: $f(d)= \alpha dt^{\eta} \sim 0.0581 t^{-0.7654}$.
The constant $\eta=-0.7654$ represents a YouTube ``memory'' factor that affects the temporal influence of videos for meme
  creation. This is used to scale graph weights in Section~\ref{sec:graph}.
  
\begin{figure}[htb]
\centering \includegraphics[angle=0, width=0.48\textwidth,height=2.0in]{fig/mem2}
\caption{\small (a) Number of unique entries returned for seven topics. (b) The fraction of unique entries over the age of the video, averaged over the seven topics.}
\label{fig:memory}
\end{figure}

\subsection{Gini phenomenon}

We have noted that YouTube answers queries using a proprietary
algorithm that strongly suggests that it uses query expansion to
enhance recall, frequently at the cost of precision. In particular,
it appears that a component of this
computation can select off-topic videos that happen to be members
of the same playlist as videos that satisfy the
query.  Further, it appears to weight these sibling videos with a
monotonic function of their view count.  Consequently, a very popular
video that happens to be in a playlist (like
``My Favorite Videos") is often selected as relevant to the query.
\eat{regardless of its title, tags, or description.}

It is common for YouTube to return query results skewed by
view counts.
However, we note that in the Iran dataset of more than 18K
videos, the 4 most popular have no near-duplicates and have nothing
to do with the topic, and likewise for 7 of the first 10.  One
has to get beyond the first 1,600 most popular videos \eat{(roughly about
the first decile of popularity)} before the likelihood of having
near-duplicates passes the average for the dataset,
which is about $0.58$ (see Figure~\ref{fig:memedata4}(a)).  Ranking by view count
leads to a ``rich-get-richer'' effect, which is independent of topic relevance.
In short, popularity is a poor proxy for relevance.

We have noted that this is a further example of the very unequal
distribution of views that characterizes this domain.  To
quantify the inequality of views-counts, we have
computed the Gini coefficient~\cite{gini1921measurement} of this data
set, and find it to have the extreme value of $0.94$, whether one looks at those
videos with near-duplicates, or those without.  The Gini coefficient,
used in economics, ranges from 0 (each video with an equal number of views)
to 1 (1 video with all of the views).  The value we
observed far exceeds the measure of inequality for the distribution of
wealth in any known country (which has its maximum at about $0.7$, for
Namibia).

% moved to parent section for joint multi-fig display
\begin{figure}[h]
\centering \includegraphics[angle=0,width=0.48\textwidth,height=2.0in]{fig/dup-prob}
\caption{Videos returned by YouTube with high view counts are less
likely to be on topic or to have near-duplicate keyframes shared with
other videos.}
\label{fig:dup-prob}
\end{figure}

\begin{figure}[h]
\centering \includegraphics[angle=0,width=0.48\textwidth,height=2.0in]{fig/dup-percent}
\caption{fraction of dataset being duped}
\label{fig:duped}
\end{figure}

%\subsection{Meme onset and reposting interval}
%
%\begin{figure}[t!]
%\centering \includegraphics[angle=0, width=0.48\textwidth,height=1.9in]{fig/histogram}
%\caption{Histogram and cumulative percentage of video memes re-posted
%  in a certain time interval by a second author, computed from Iran dataset B.}
%\label{fig:histogram}
%\end{figure}
%
%Figure~\ref{fig:histogram} shows the expected time interval before a
%new visual meme is discovered and re-posted after its initial upload.
%The left $y$-axis shows the number of meme video that were first
%reposted in a given time interval, and the right $y$-axis shows the
%cumulative percentage.  The statistics are computed from the Iran
%topic dataset (B), based on approximately 2300 meme video that have
%at least 10 duplications by other authors.  The results show
%that more than half of the memes are re-posted within 3 hours of
%their initial upload, and over 70\% are re-posted the same day. The
%graph also shows a secondary peak at the granularity of a weak.

\secmoveup
\subsection{Visual meme modeling}
\label{sec:twoviews} \textmoveup

We start by presenting two complementary views on visual memes, in order to build models for this large-scale media gist in networked
social interactions.

In one view we treat memes as {\em links} -- where videos and people are interacting entities (nodes) in a dynamic network. Each re-posted
meme image is an explicit statement of mutual awareness, or a relevance statement on a mutually interested subject, just like hyperlinks on
the world-wide web. Here visual memes behave like the {\em RT} twitter tags (retweet verbatim)~\cite{Kwak10twitter} for inferencing
relationship between authors.
%Here, we view memes as links that connect among content and people, which collectively evolve in shared event context and
%co-develop the emerging themes.

In the other view we treat visual memes as {\em words} -- where videos are documents that contain them, and memes are part of a shared
vocabulary that people use around the same event, where Figure~\ref{fig:memedata4} shows that visual memes behave like words statistically. The
visual meme vocabulary expresses additional concepts not captured in words (text). The memes (visual words) and textual words jointly
define the topics and trends in an event, through which summarization, monitoring and exploration are possible. This is closer to the Meme
Tracker~\cite{leskovec2009meme} presentation, where meme phrases are presented as a set of streams flowing over time.

We begin by defining notations to represent the event media stream to facilitate modeling in both views. We start by using notations from
the document view, and then adapt it to represent the network view. Denote a video as a multimedia document $d_m$ in event collection
${\cal D}$, with $m=1,\ldots,M$. Each video is authored (uploaded) by a user $a(d_m)$ at time $t(d_m)$, where $a(d_m)$ takes its value from
the set of users ${\cal A}=\{a_r, r=1,\ldots,R\}$. Each document $d_m$ contains a collection of words, $\{w_{m1}, w_{m2},\ldots,
w_{mN_m}\}$, each of which can be textual terms (from the title, description, comments, tags) $w_t$ and visual terms $w_v$, from the
respective word- and meme- dictionaries, ${\cal V}_t$ and ${\cal V}_v$. In the networked view, the nodes consist of distinct documents
$d_m,~m=1,\ldots,M$ or individual authors $a_r,~r=1,\ldots,R$, and memes are treated as time-sensitive edges $e_{ij}$ with creation time
$t(e_{ij})$, where $i,j$ are over the dimensions of the graph.
